# Supplementary material for: Safe Planning in Dynamic Environments using Conformal Prediction
Source: arXiv:2210.10254 source file (2023-06-08)
Supplement: Supplementary file 1 [file appendix.tex]

\section{Needed?}
